# Supplementary material for: $\beta$-DARTS++: Bi-level Regularization for Proxy-robust Differentiable Architecture Search
Source: arXiv:2301.06393 source file (2023-01-16)
Supplement: Supplementary file 1 [file supp_file.tex]

\documentclass[10pt,journal,compsoc]{IEEEtran}
%
% If IEEEtran.cls has not been installed into the LaTeX system files,
% manually specify the path to it like:
% \documentclass[10pt,journal,compsoc]{../sty/IEEEtran}

% Some very useful LaTeX packages include:
% (uncomment the ones you want to load)

% *** MISC UTILITY PACKAGES ***
%
%\usepackage{ifpdf}
% Heiko Oberdiek's ifpdf.sty is very useful if you need conditional
% compilation based on whether the output is pdf or dvi.
% usage:
% \ifpdf
%   % pdf code
% \else
%   % dvi code
% \fi
% The latest version of ifpdf.sty can be obtained from:
% http://www.ctan.org/pkg/ifpdf
% Also, note that IEEEtran.cls V1.7 and later provides a builtin
% \ifCLASSINFOpdf conditional that works the same way.
% When switching from latex to pdflatex and vice-versa, the compiler may
% have to be run twice to clear warning/error messages.

% *** CITATION PACKAGES ***
%
\ifCLASSOPTIONcompsoc
  % IEEE Computer Society needs nocompress option
  % requires cite.sty v4.0 or later (November 2003)
  \usepackage[nocompress]{cite}
\else
  % normal IEEE
  \usepackage{cite}
\fi
% cite.sty was written by Donald Arseneau
% V1.6 and later of IEEEtran pre-defines the format of the cite.sty package
% \cite{} output to follow that of the IEEE. Loading the cite package will
% result in citation numbers being automatically sorted and properly
% "compressed/ranged". e.g., [1], [9], [2], [7], [5], [6] without using
% cite.sty will become [1], [2], [5]--[7], [9] using cite.sty. cite.sty's
% \cite will automatically add leading space, if needed. Use cite.sty's
% noadjust option (cite.sty V3.8 and later) if you want to turn this off
% such as if a citation ever needs to be enclosed in parenthesis.
% cite.sty is already installed on most LaTeX systems. Be sure and use
% version 5.0 (2009-03-20) and later if using hyperref.sty.
% The latest version can be obtained at:
% http://www.ctan.org/pkg/cite
% The documentation is contained in the cite.sty file itself.
%
% Note that some packages require special options to format as the Computer
% Society requires. In particular, Computer Society  papers do not use
% compressed citation ranges as is done in typical IEEE papers
% (e.g., [1]-[4]). Instead, they list every citation separately in order
% (e.g., [1], [2], [3], [4]). To get the latter we need to load the cite
% package with the nocompress option which is supported by cite.sty v4.0
% and later. Note also the use of a CLASSOPTION conditional provided by
% IEEEtran.cls V1.7 and later.

% *** GRAPHICS RELATED PACKAGES ***
%
\ifCLASSINFOpdf
  % \usepackage[pdftex]{graphicx}
  % declare the path(s) where your graphic files are
  % \graphicspath{{../pdf/}{../jpeg/}}
  % and their extensions so you won't have to specify these with
  % every instance of \includegraphics
  % \DeclareGraphicsExtensions{.pdf,.jpeg,.png}
\else
  % or other class option (dvipsone, dvipdf, if not using dvips). graphicx
  % will default to the driver specified in the system graphics.cfg if no
  % driver is specified.
  % \usepackage[dvips]{graphicx}
  % declare the path(s) where your graphic files are
  % \graphicspath{{../eps/}}
  % and their extensions so you won't have to specify these with
  % every instance of \includegraphics
  % \DeclareGraphicsExtensions{.eps}
\fi
\usepackage[pagebackref,breaklinks,colorlinks]{hyperref}
\usepackage{multirow}
\usepackage{graphicx}
\usepackage{amssymb}
\usepackage{booktabs}
\usepackage{xcolor}
\usepackage{amsmath,mathtools}
\usepackage{array}
\usepackage{ragged2e}
% correct bad hyphenation here
\hyphenation{op-tical net-works semi-conduc-tor}
% \captionsetup[table]{justification=centering}
\usepackage{array, caption, threeparttable}
% \usepackage[font=small,labelfont=bf,labelsep=none]{caption}
%表格编号Table 1 可以加粗显示

\begin{document}
%
% paper title
% Titles are generally capitalized except for words such as a, an, and, as,
% at, but, by, for, in, nor, of, on, or, the, to and up, which are usually
% not capitalized unless they are the first or last word of the title.
% Linebreaks \\ can be used within to get better formatting as desired.
% Do not put math or special symbols in the title.
% \title{Bare Demo of IEEEtran.cls for\\ IEEE Computer Society Journals} 
\title{$\beta$-DARTS++: Bi-level Regularization for Proxy-robust Differentiable Architecture Search}

\author{
% Peng Ye\textsuperscript{1}, Tong He\textsuperscript{2}, Baopu Li\textsuperscript{3}, Tao Chen\textsuperscript{1}\thanks{ Corresponding author (eetchen@fudan.edu.cn)}~, Lei Bai\textsuperscript{2}, Wanli Ouyang\textsuperscript{2,4}
Peng Ye, Tong He, Baopu Li, Tao Chen, Lei Bai, Wanli Ouyang
% Michael~Shell,~\IEEEmembership{Member,~IEEE,}
%         John~Doe,~\IEEEmembership{Fellow,~OSA,}
%         and~Jane~Doe,~\IEEEmembership{Life~Fellow,~IEEE}% <-this % stops a space
\IEEEcompsocitemizethanks{\IEEEcompsocthanksitem Peng Ye and Tao Chen are with the School of Information Science and Technology, Fudan University, Shanghai, China \\
% note need leading \protect in front of \\ to get a newline within \thanks as
% \\ is fragile and will error, could use \hfil\break instead.
E-mail: \{20110720039, eetchen\}@fudan.edu.cn
\IEEEcompsocthanksitem Tong He, Lei Bai and Wanli Ouyang are with the Shanghai AI Laboratory, Shanghai, China.
\IEEEcompsocthanksitem Baopu Li is with the Oracle Health and AI, Oracle, USA.
\IEEEcompsocthanksitem Work performed when Peng Ye is intern of Shanghai AI Laboratory, China. Tao Chen is the corresponding author.}% <-this % stops an unwanted space
% \thanks{Manuscript received xx xx, xx; revised xx xx, xx.}
}

% note the % following the last \IEEEmembership and also \thanks - 
% these prevent an unwanted space from occurring between the last author name
% and the end of the author line. i.e., if you had this:
% 
% \author{....lastname \thanks{...} \thanks{...} }
%                     ^------------^------------^----Do not want these spaces!
%
% a space would be appended to the last name and could cause every name on that
% line to be shifted left slightly. This is one of those "LaTeX things". For
% instance, "\textbf{A} \textbf{B}" will typeset as "A B" not "AB". To get
% "AB" then you have to do: "\textbf{A}\textbf{B}"
% \thanks is no different in this regard, so shield the last } of each \thanks
% that ends a line with a % and do not let a space in before the next \thanks.
% Spaces after \IEEEmembership other than the last one are OK (and needed) as
% you are supposed to have spaces between the names. For what it is worth,
% this is a minor point as most people would not even notice if the said evil
% space somehow managed to creep in.

% The paper headers
\markboth{Journal of \LaTeX\ Class Files,~Vol.~14, No.~8, August~2015}%
{Shell \MakeLowercase{\textit{et al.}}: Bare Demo of IEEEtran.cls for Computer Society Journals}
\maketitle

% To allow for easy dual compilation without having to reenter the
% abstract/keywords data, the \IEEEtitleabstractindextext text will
% not be used in maketitle, but will appear (i.e., to be "transported")
% here as \IEEEdisplaynontitleabstractindextext when the compsoc 
% or transmag modes are not selected <OR> if conference mode is selected 
% - because all conference papers position the abstract like regular
% papers do.
\IEEEdisplaynontitleabstractindextext
% \IEEEdisplaynontitleabstractindextext has no effect when using
% compsoc or transmag under a non-conference mode.

% For peer review papers, you can put extra information on the cover
% page as needed:
% \ifCLASSOPTIONpeerreview
% \begin{center} \bfseries EDICS Category: 3-BBND \end{center}
% \fi
%
% For peerreview papers, this IEEEtran command inserts a page break and
% creates the second title. It will be ignored for other modes.
\IEEEpeerreviewmaketitle

\begin{figure*}[t]
\hsize=\textwidth
\centering
\hspace{-0.2in}
\centering
\includegraphics[width=2.0\columnwidth]{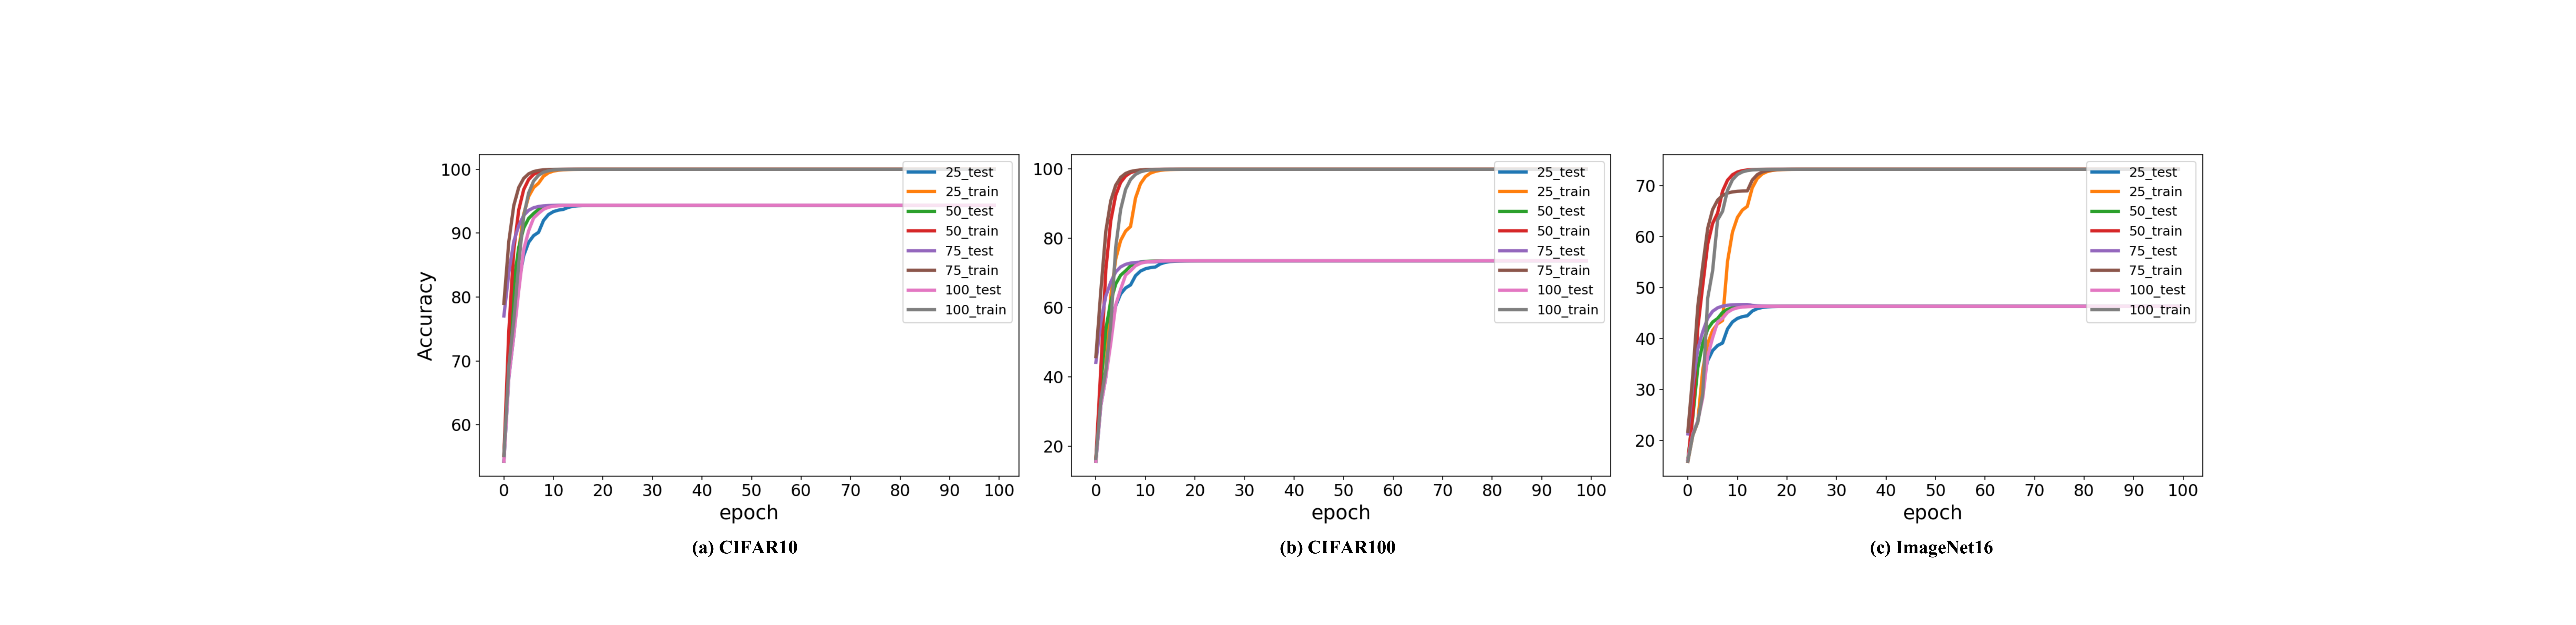}
\vspace{-6pt}
\caption{Accuracies of different datasets of $\beta$-DARTS with different max weights (i.e., 25/50/75/100) on NAS-Bench-201 benchmark. The curve is smoothed with a coefficient of 0.5. Note that we only search once on CIFAR-10 dataset and report the results of different datasets.}
\label{fig:7}
% \vspace{-3pt}	
\end{figure*}
% \vspace{2mm}
% }]

\appendices
\section{}
\subsection{Derivation of Eq.~(8) in The Main Text.}
For the optimization process of architecture parameters, we utilize the following unified formulas to represent the single-step update with/without regularization.
\begin{equation} \label{eqn20}
  \begin{split}
    &\alpha_{k}^{t+1} \leftarrow \alpha_{k}^{t}-\eta_{\alpha} \nabla_{\alpha_{k}} \mathcal{L}_{val} \\
    &\bar{\alpha}_{k}^{t+1} \leftarrow \alpha_{k}^{t}-\eta_{\alpha} \nabla_{\alpha_{k}} \mathcal{L}_{val}-\eta_{\alpha} \lambda F\left(\alpha_{k}^{t}\right)
  \end{split}
  \vspace{-6pt}
\end{equation}

For the single-step update without regularization, via $\alpha$ in Eq.~(\ref{eqn20}), we can compute the softmax-activated architecture parameters $\beta$ as
\begin{equation} \label{eqn21}
  \begin{split}
    \beta_{k}^{t+1}=\frac{\exp \left(\alpha_{k}^{t+1} \right)}{\sum_{k^{\prime}=1}^{\left | \mathcal{O}\right |}  \exp \left(\alpha_{k^{\prime}}^{t+1}\right)}
  \end{split}
  \vspace{-6pt}
\end{equation}

For the single-step update with regularization, based on $\bar{\alpha}$ in Eq.~(\ref{eqn20}), we can further compute the softmax-activated architecture parameters $\bar{\beta}$ as
% \begin{center}
\begin{equation} \label{eqn22}
\small
  \begin{split}
    &\bar{\beta}_{k}^{t+1}=\frac{\exp \left(\bar{\alpha}_{k}^{t+1} \right)}{\sum_{k^{\prime}=1}^{\left | \mathcal{O}\right |} \exp \left(\bar{\alpha}_{k^{\prime}}^{t+1} \right)} \\
    &=\frac{\exp \left(-\lambda \eta_{\alpha}F(\alpha_k^{t})\right)\exp \left(\alpha_{k}^{t+1} \right)}{\sum_{k^{\prime}=1}^{\left | \mathcal{O}\right |} \exp \left(-\lambda \eta_{\alpha}F(\alpha_{k^{\prime}}^{t})\right) \exp \left(\alpha_{k^{\prime}}^{t+1} \right)} \\
    &=\frac{\exp \left(\alpha_{k}^{t+1} \right)}{\sum_{k^{\prime}=1}^{\left | \mathcal{O}\right |} \frac{\exp \left(-\lambda \eta_{\alpha}F(\alpha_{k^{\prime}}^{t})\right)}{\exp \left(-\lambda \eta_{\alpha}F(\alpha_k^{t})\right)} \exp \left(\alpha_{k^{\prime}}^{t+1}\right)} \\
    &=\frac{\exp \left(\alpha_{k}^{t+1} \right)}{\sum_{k^{\prime}=1}^{\left | \mathcal{O}\right |} \left[\exp \left(F(\alpha_{k}^{t})-F(\alpha_{k^{\prime}}^{t})\right)\right]^{\lambda \eta_{\alpha}} \exp \left(\alpha_{k^{\prime}}^{t+1} \right)}
  \end{split}
  \vspace{-6pt}
\end{equation}
% \end{center}

Then, dividing Eq.~(\ref{eqn22}) by Eq.~(\ref{eqn21}), we can obtain the influence of $\alpha$ with regularization on $\beta$.
\begin{equation} \label{eqn23}
\footnotesize
  \begin{split}
    \frac{\bar{\beta}_{k}^{t+1}}{\beta_{k}^{t+1}}=\frac{\sum_{k^{\prime}=1}^{\left | \mathcal{O}\right |} \exp \left(\alpha_{k^{\prime}}^{t+1}\right)}{\sum_{k^{\prime}=1}^{\left | \mathcal{O}\right |} \left[\exp \left(F(\alpha_{k}^{t})-F(\alpha_{k^{\prime}}^{t})\right)\right]^{\lambda \eta_{\alpha}} \exp \left(\alpha_{k^{\prime}}^{t+1}\right)}
  \end{split}
  \vspace{6pt}
\end{equation}

% you can choose not to have a title for an appendix
% if you want by leaving the argument blank
\section{}
\subsection{More Results about The Search Trajectories.}
In Fig.~\ref{fig:7}, we show the search trajectories of different datasets of $\beta$-DARTS with different max weights (i.e., 25/50/75/100) on NAS-Bench-201 benchmark. Similarly, we can see that: (1) the performance collapse issue is well solved and $\beta$-DARTS has a stable search process; (2) the architecture found on CIFAR-10 performs well on CIFAR-10, CIFAR-100 and ImageNet; (3) the search process of different datasets reach the optimal point at an early stage but in different epochs; (4) different runs of searching under different max weight always find the same optimal solution.
\subsection{Effectiveness and Efficiency of Proposed Alpha Standard Deviation Based Criteria.}
In Table~\ref{tab:adaptive-epoch1}, we present the search results from multiple independent runs via the proposed alpha standard deviation based criterion. As we can see, all the proposed criteria 1, 2 and 3 can automatically decide the optimal epoch of searching under different proxy data. And from criteria 1 until criteria 3, the end epoch becomes larger, while the search performance usually becomes better. In particular, criteria 2 and criteria 3 can achieve almost the same performance with that of searching until the last epoch, while using much fewer epochs, verifying the effectiveness and efficiency of the alpha standard deviation based criteria. 
\subsection{Wide Range of The Optimal Weight.}
In Fig.~\ref{fig:8}, we further show the influence of different max weights on the searching results of $\beta$-DARTS on common DARTS search space on CIFAR-10 and CIFAR-100. Also, the performance of original DARTS~\cite{darts} (i.e., 97.00 on CIFAR-10 and 82.46 on CIFAR-100) is improved on a wide range of max weights and the optimal searching result is obtained on multiple values of max weights.

%-------------------------------------------------------------------------
\begin{table*}[t]
\caption{The optimal epoch and corresponding search performance indicated by different Criteria. Criteria 1/2/3 denotes the alpha standard deviation based criteria for adaptive search, and Criteria 4 means searching until the last epoch.} %on NAS-Bench-201 benchmark.}
% \begin{center}
\vspace{-3pt}
\label{tab:adaptive-epoch1}
% \resizebox{\linewidth}{!}{
% \resizebox{\textwidth}{6mm}{
\begin{tabular}{ccccccc}
\hline
\multirow{2}{*}{\begin{tabular}[c]{@{}c@{}}Partial \\ data\end{tabular}} & \multicolumn{2}{c}{Criteria 1/2/3/4}   & \multicolumn{2}{c}{Criteria 1/2/3/4}   & \multicolumn{2}{c}{Criteria 1/2/3/4}  \\ \cline{2-7} 
& End epoch    & C10 val                 & End epoch    & C10 val                 & End epoch   & C10 val                 \\ \hline
100\%                                                                    & 8/15/60/100  & 91.50/91.55/91.55/91.55 & 8/13/50/100  & 91.55/91.55/91.55/91.55 & 8/20/56/100 & 91.61/91.55/91.55/91.55 \\
75\%                                                                     & 9/16/42/100  & 91.50/91.55/91.55/91.55 & 10/27/31/100 & 91.55/91.55/91.55/91.55 & 7/16/37/100 & 91.28/91.50/91.55/91.55 \\
50\%                                                                     & 10/14/38/100 & 91.55/91.55/91.55/91.55 & 8/9/34/100   & 91.55/91.55/91.55/91.55 & 9/11/27/100 & 91.61/91.61/91.61/91.55 \\
25\%                                                                     & 5/12/25/100  & 90.98/91.55/91.55/91.55 & 7/10/25/100  & 91.34/91.44/91.53/91.53 & 1/9/21/100  & 75.21/90.54/91.61/91.61 \\
20\%                                                                     & 7/11/24/100  & 90.94/91.42/91.61/91.61 & 7/9/20/100   & 91.48/91.48/91.48/91.48 & 7/8/28/100  & 89.81/89.81/91.53/91.53 \\
10\%                                                                     & 5/9/31/100   & 89.76/90.30/90.30/90.02 & 2/7/12/100   & 87.61/89.59/90.69/90.18 & 2/8/13/100  & 89.63/89.76/90.45/89.48 \\
5\%                                                                      & 2/4/7/100    & 68.01/88.24/88.24/89.16 & 2/6/11/100   & 89.55/91.07/91.35/89.65 & 2/6/13/100  & 89.55/91.07/91.35/89.65 \\
2\%                                                                      & 1/3/6/100    & 88.79/90.11/90.11/90.11 & 1/4/9/100    & 88.79/90.02/90.02/90.07 & 1/4/10/100  & 88.95/89.93/90.07/90.02 \\
1\%                                                                      & 1/2/7/100    & 88.10/88.65/90.45/90.45 & 1/3/7/100    & 88.10/89.13/90.30/90.45 & 1/3/8/100   & 88.10/88.10/90.45/90.12 \\ \hline
\end{tabular}
% }
% \end{center}
% \vspace{-12pt}
\end{table*}
%-------------------------------------------------------------------------
\begin{figure*}[t] 
	\centering
	\includegraphics[width=1.0\linewidth]{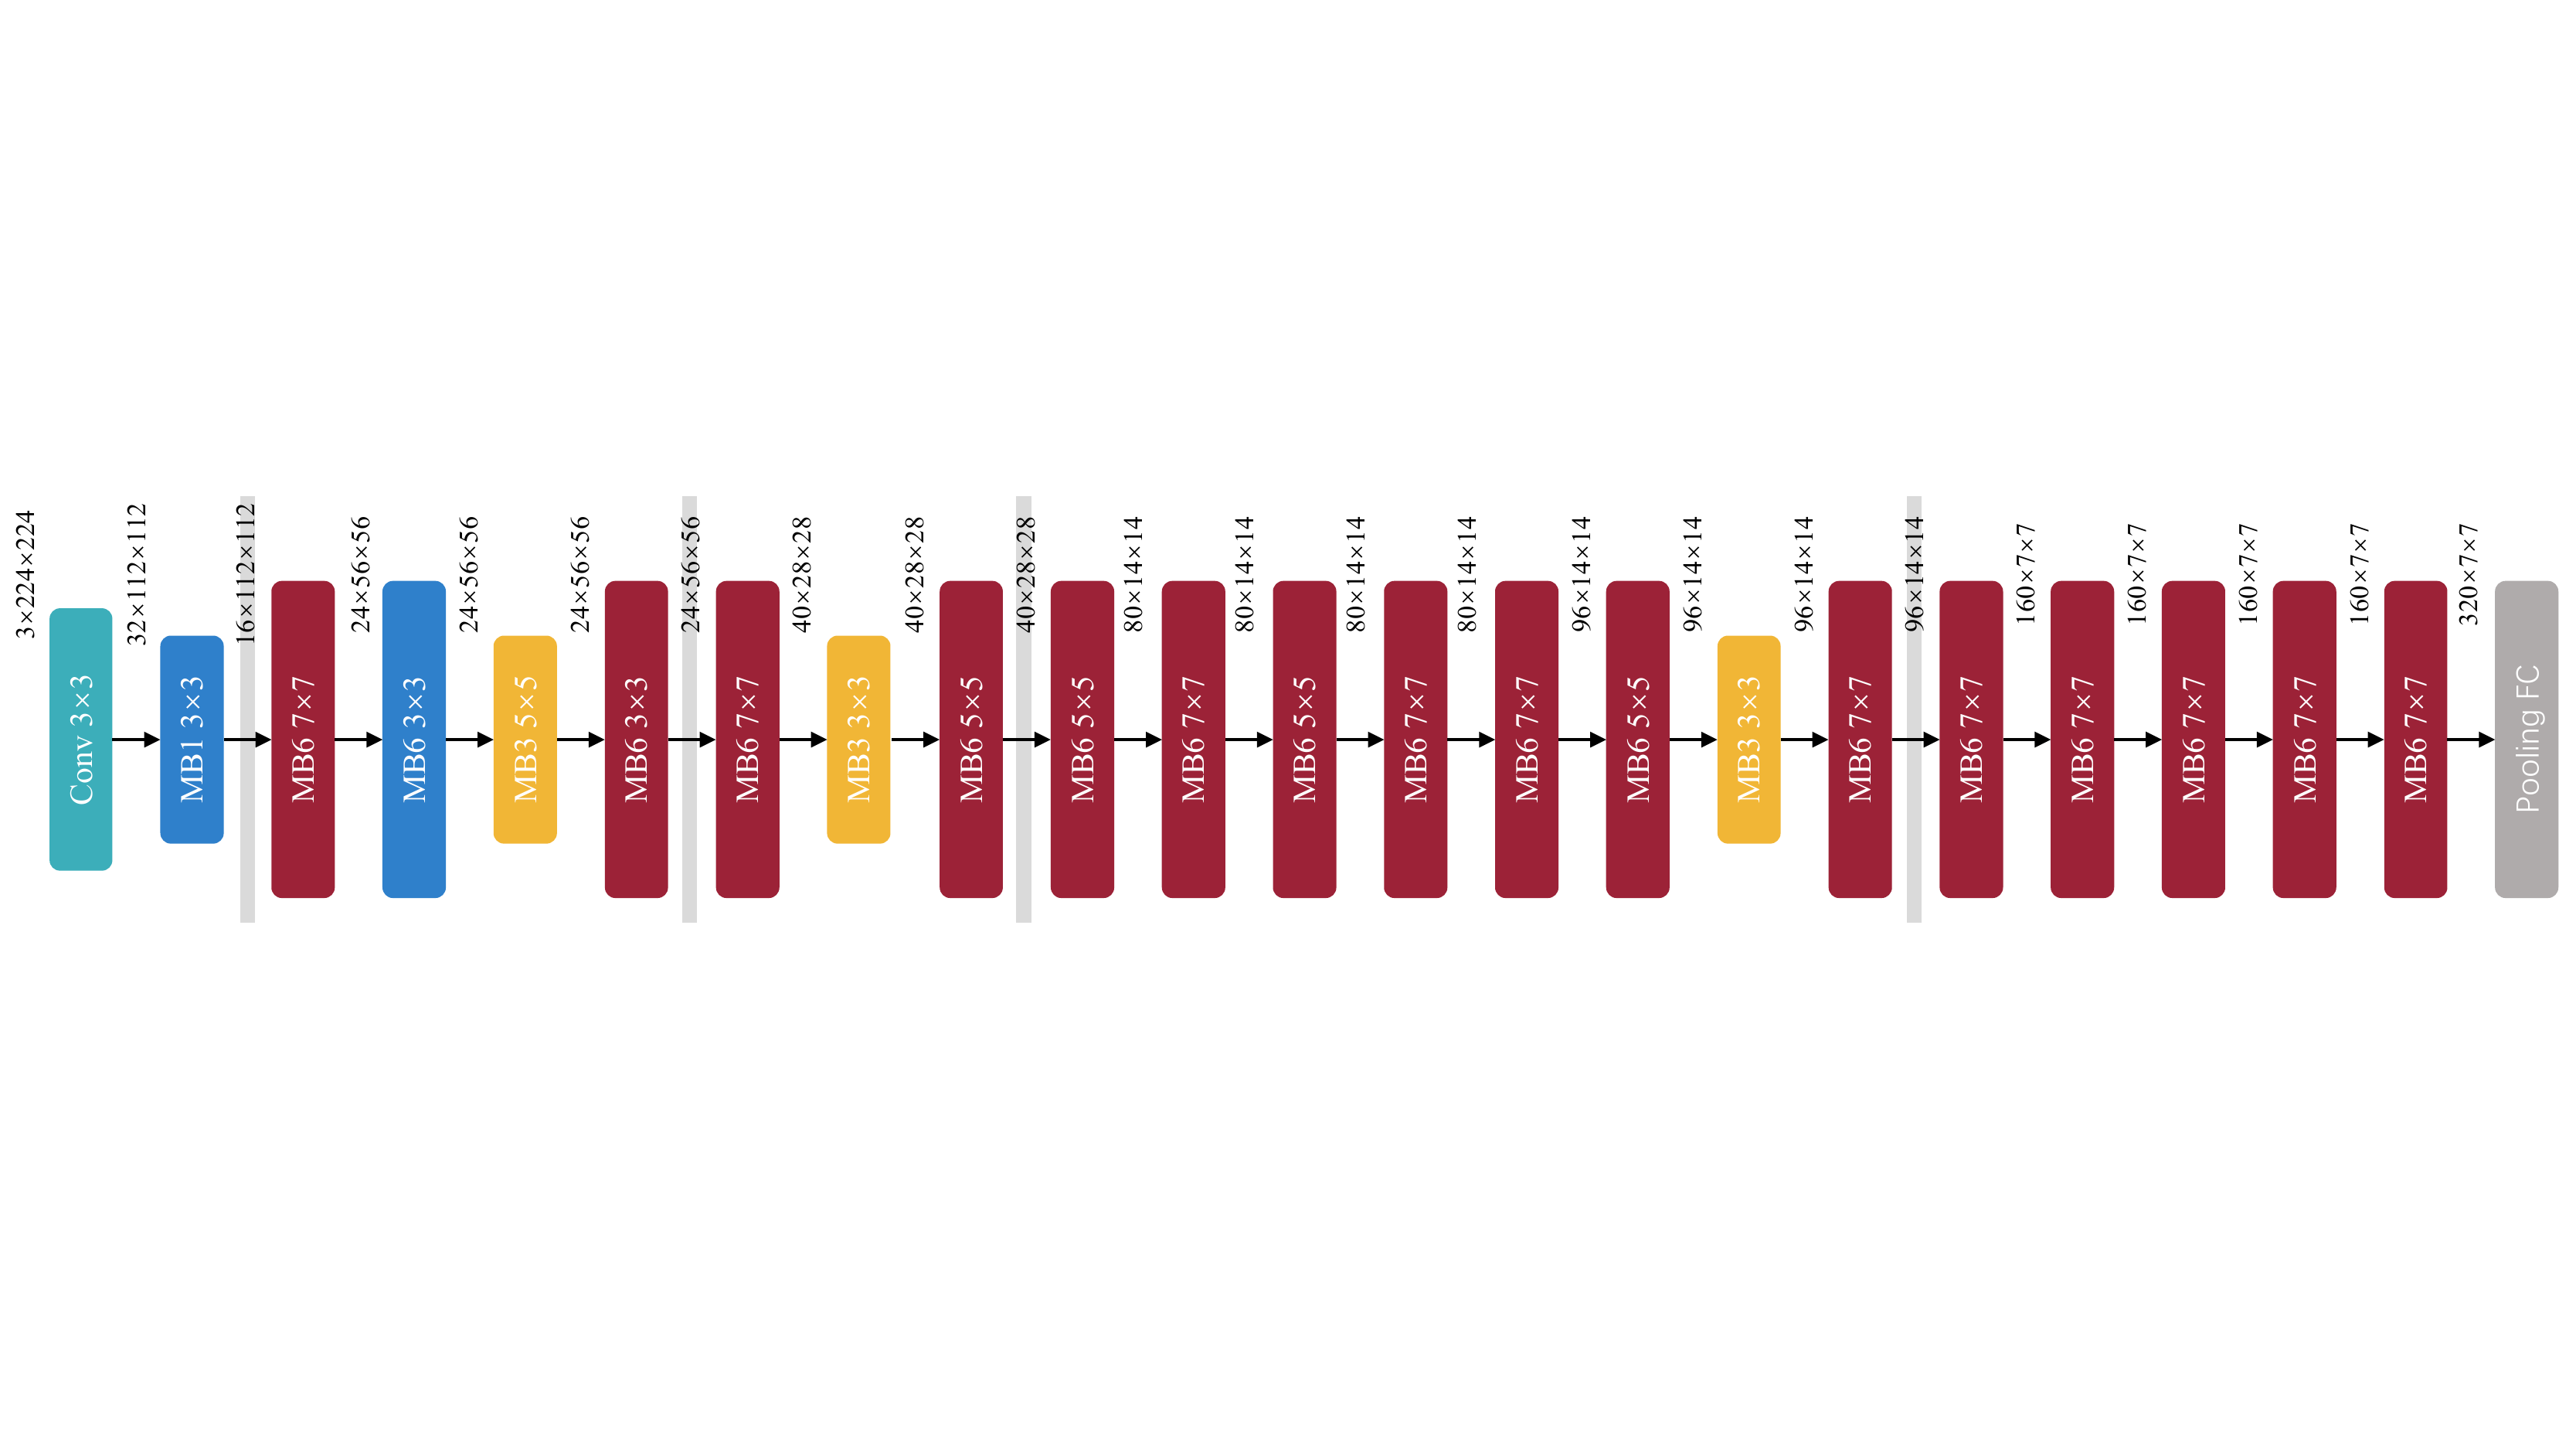}
    \vspace{-20pt}
	\caption{The architecture discovered by $\beta$-DARTS on MobileNet search space on ImageNet dataset. "MB3" and "MB6" denotes the mobile inverted bottleneck convolution layer with an expansion ratio of 3 and 6 respectively. And 3$\times$3, 5$\times$5 and 7$\times$7 mean the convolution kernel size.}
	\label{fig:mobile}
	\vspace{-12pt}	
\end{figure*}

\begin{figure}[t] 
	\centering
	\includegraphics[width=3.0in]{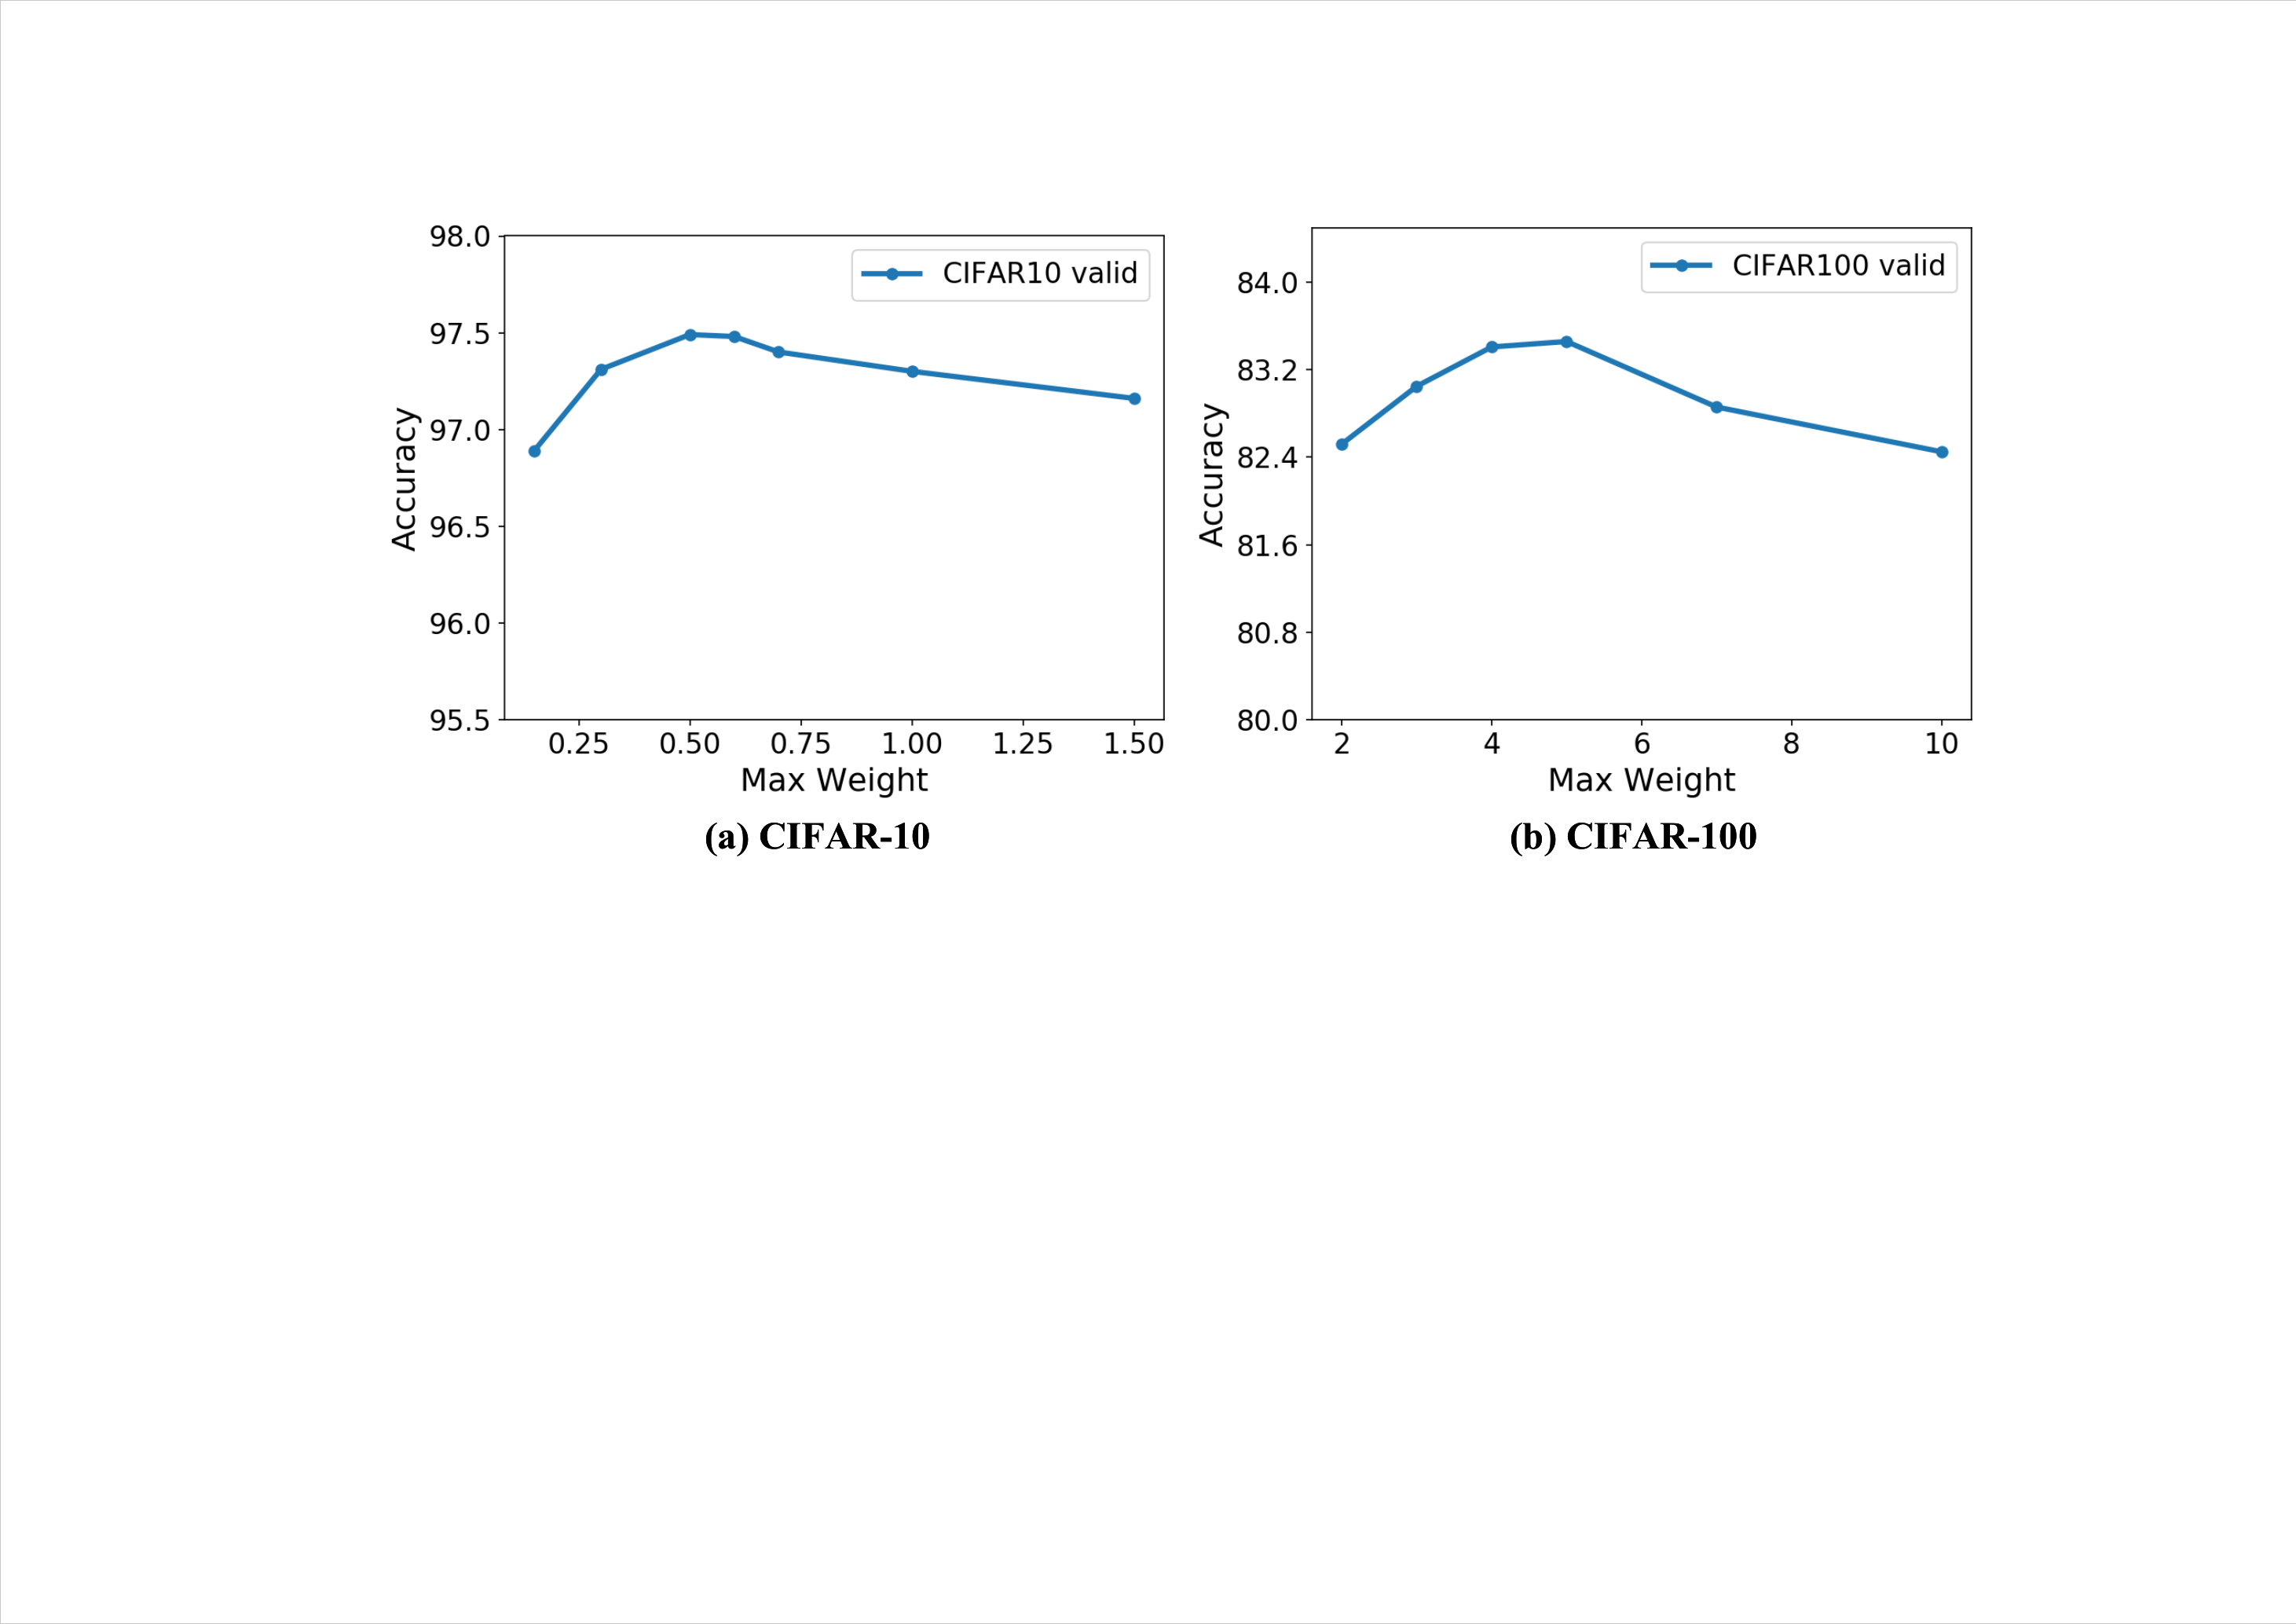}
    \vspace{-6pt}
	\caption{The effect of different max weights of linearly increasing weighting on the searching results of DARTS search space.}
	\label{fig:8}
	\vspace{-12pt}	
\end{figure}

\section{}
\subsection{Visualization of All The Searched Architectures on DARTS Search Space.}
In Fig.~\ref{fig:12} and Fig.~\ref{fig:13}, we visualize the genotypes of normal and reduction cells searched on common DARTS search space on CIFAR-10 and CIFAR-100 datasets respectively. We can see that all models searched by 3 runs of independent searching of $\beta$-DARTS will not be dominated by the parametric-free operators like skip-connection.

\subsection{Visualization of The Searched Model on MobileNet Search Space.}
In Fig.~\ref{fig:mobile}, we visualize the architecture found by $\beta$-DARTS on MobileNet search space on ImageNet dataset. As we can see, the architecture is mainly composed of MB6 7$\times$7 and will not be dominated by skip-connection.

\begin{figure*}[t] 
	\centering
	\includegraphics[width=1.0\linewidth]{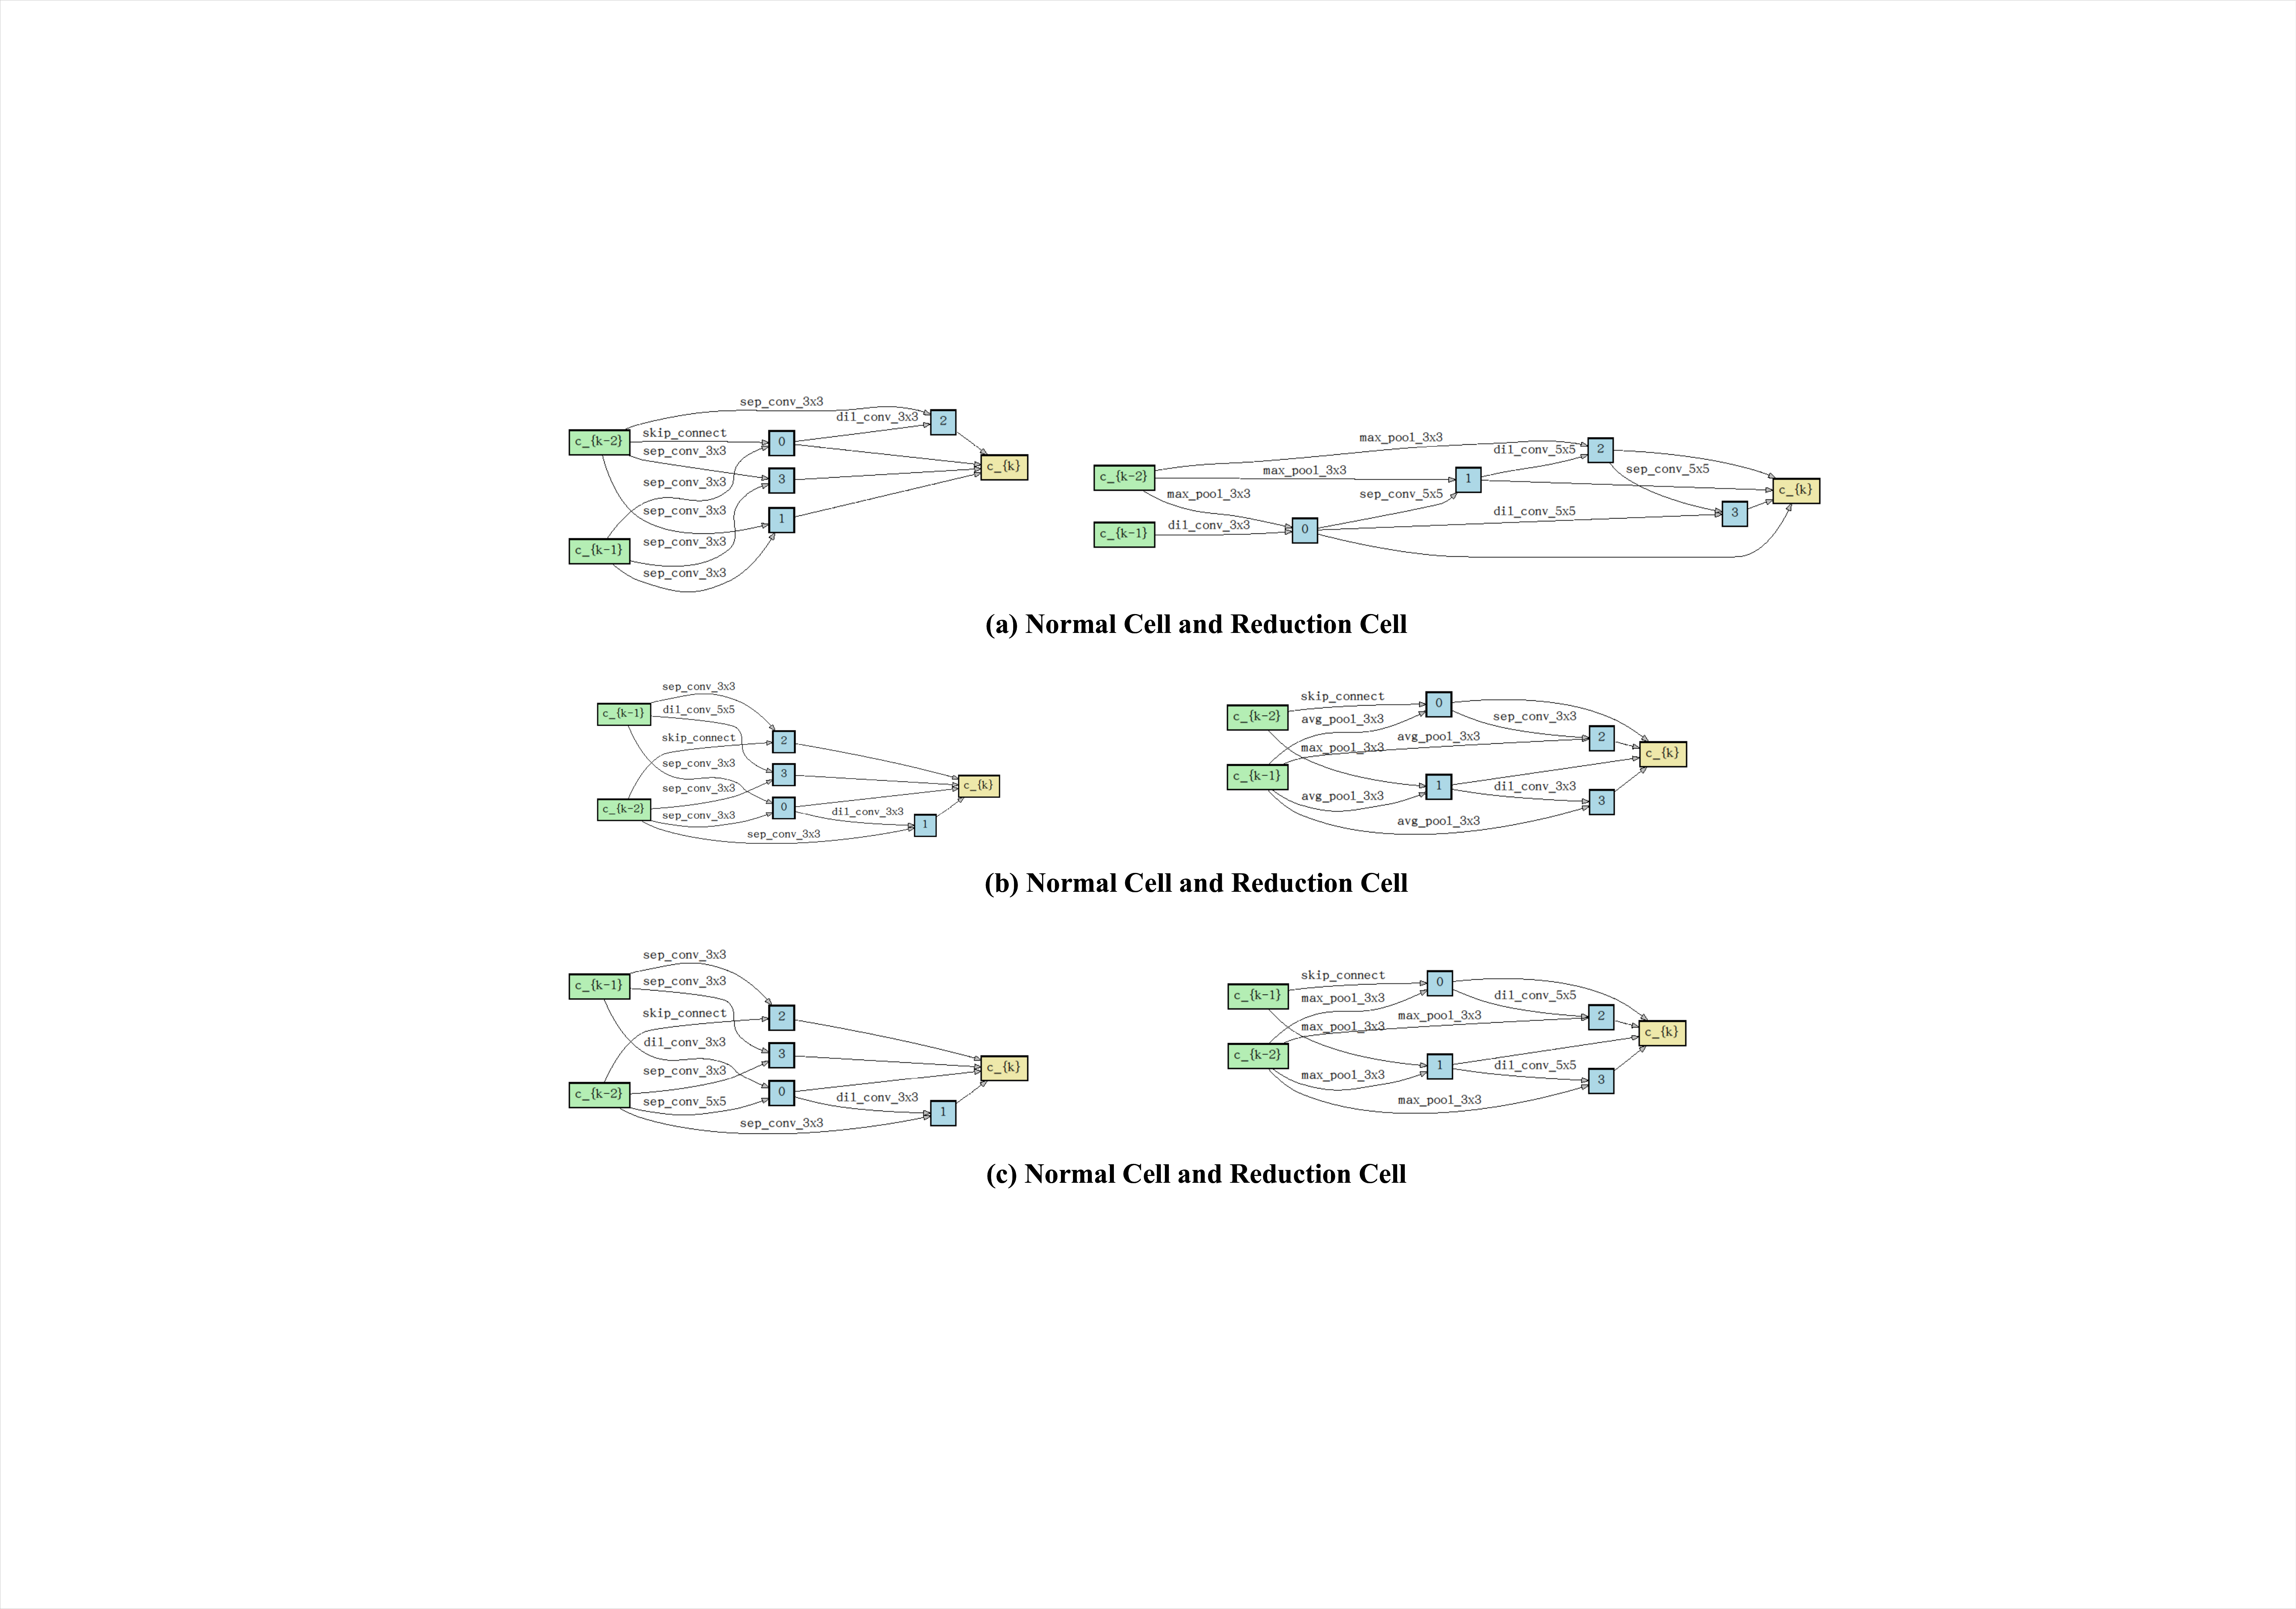}
	\caption{Normal cell (left) and Reduction cell (right) discovered by $\beta$-DARTS on common DARTS search space on CIFAR-10 dataset. (a), (b) and (c) denote the found genotypes of the 3 runs of independent searching.}
	\label{fig:12}
	\vspace{-12pt}	
\end{figure*}

\begin{figure*}[t] 
	\centering
	\includegraphics[width=1.0\linewidth]{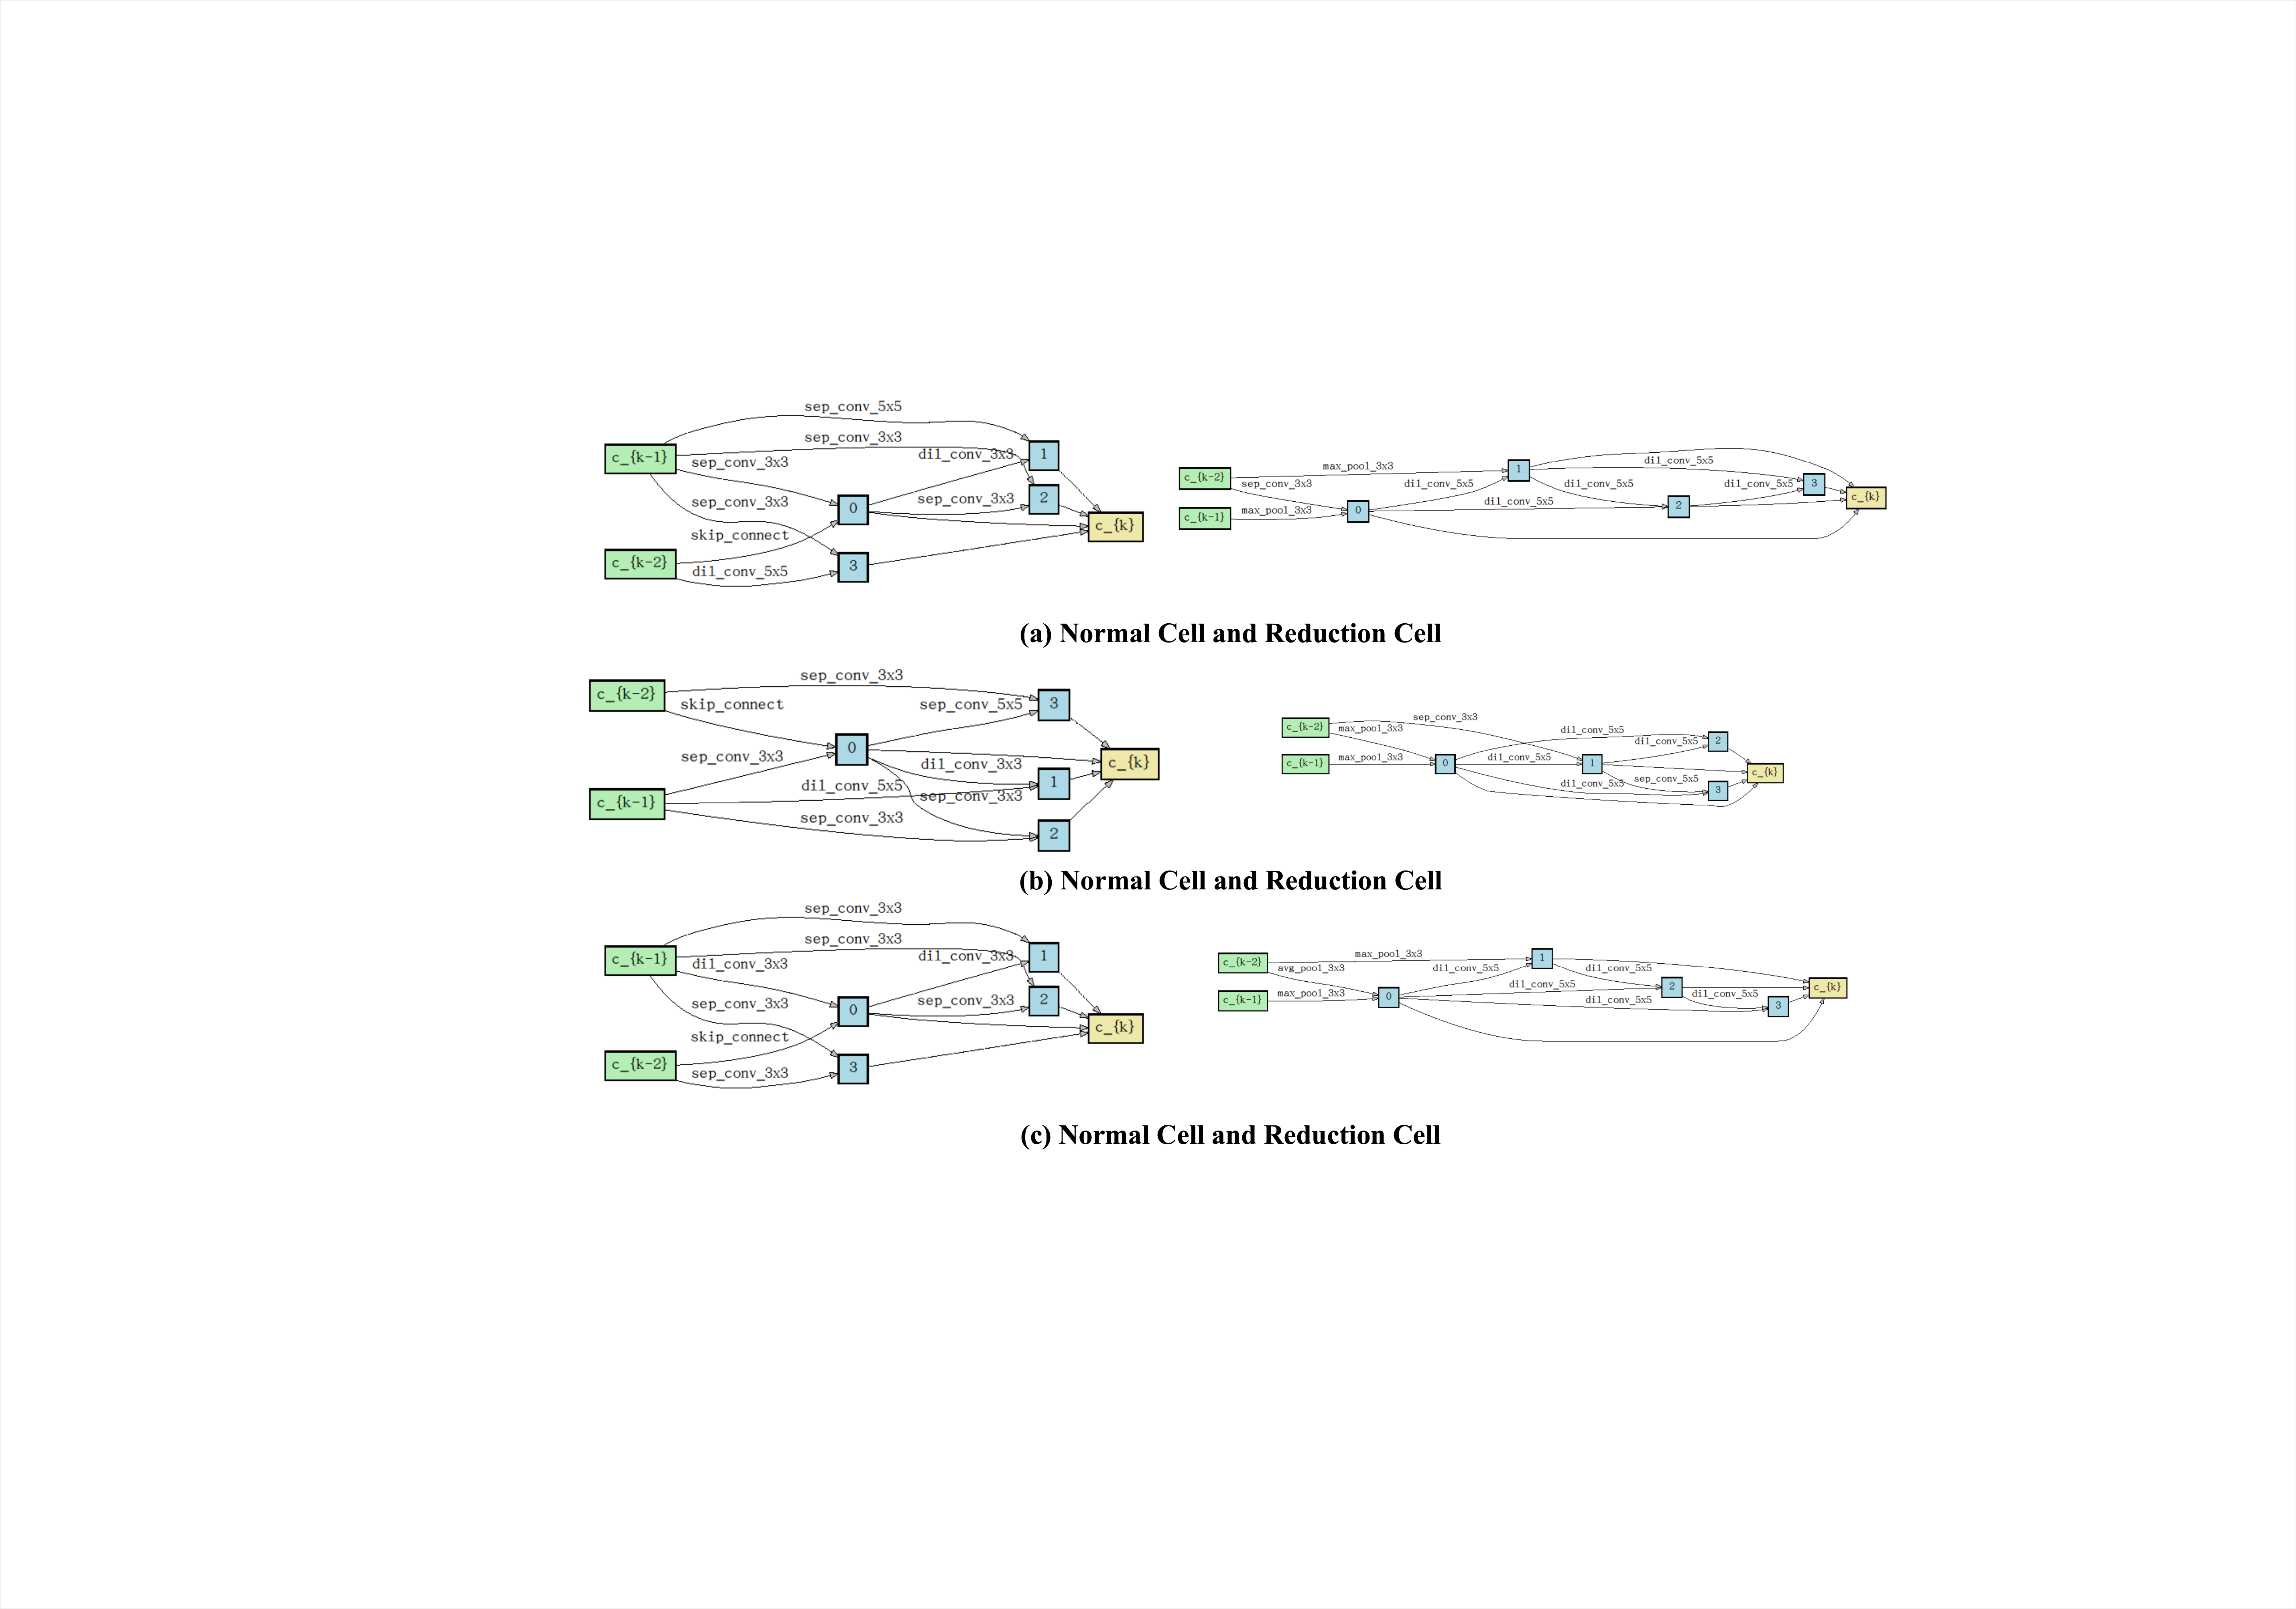}
	\caption{Normal cell (left) and Reduction cell (right) discovered by $\beta$-DARTS on common DARTS search space on CIFAR-100. (a), (b) and (c) denote the found genotypes of 3 runs of independent searching.}
	\label{fig:13}
	\vspace{-12pt}	
\end{figure*}

% % use section* for acknowledgment
% \ifCLASSOPTIONcompsoc
%   % The Computer Society usually uses the plural form
%   \section*{Acknowledgments}
% \else
%   % regular IEEE prefers the singular form
%   \section*{Acknowledgment}
% \fi

% The authors would like to thank...

% Can use something like this to put references on a page
% by themselves when using endfloat and the captionsoff option.
\ifCLASSOPTIONcaptionsoff
  \newpage
\fi

% trigger a \newpage just before the given reference
% number - used to balance the columns on the last page
% adjust value as needed - may need to be readjusted if
% the document is modified later
%\IEEEtriggeratref{8}
% The "triggered" command can be changed if desired:
%\IEEEtriggercmd{\enlargethispage{-5in}}

% references section

% can use a bibliography generated by BibTeX as a .bbl file
% BibTeX documentation can be easily obtained at:
% http://mirror.ctan.org/biblio/bibtex/contrib/doc/
% The IEEEtran BibTeX style support page is at:
% http://www.michaelshell.org/tex/ieeetran/bibtex/
\bibliographystyle{IEEEtran}
% argument is your BibTeX string definitions and bibliography database(s)
\bibliography{main_paper}
\end{document}
